# Supplementary material for: New Lower Bound and Algorithms for Online Geometric Hitting Set Problem
Source: arXiv:2409.11166 source file (2024-10-01)

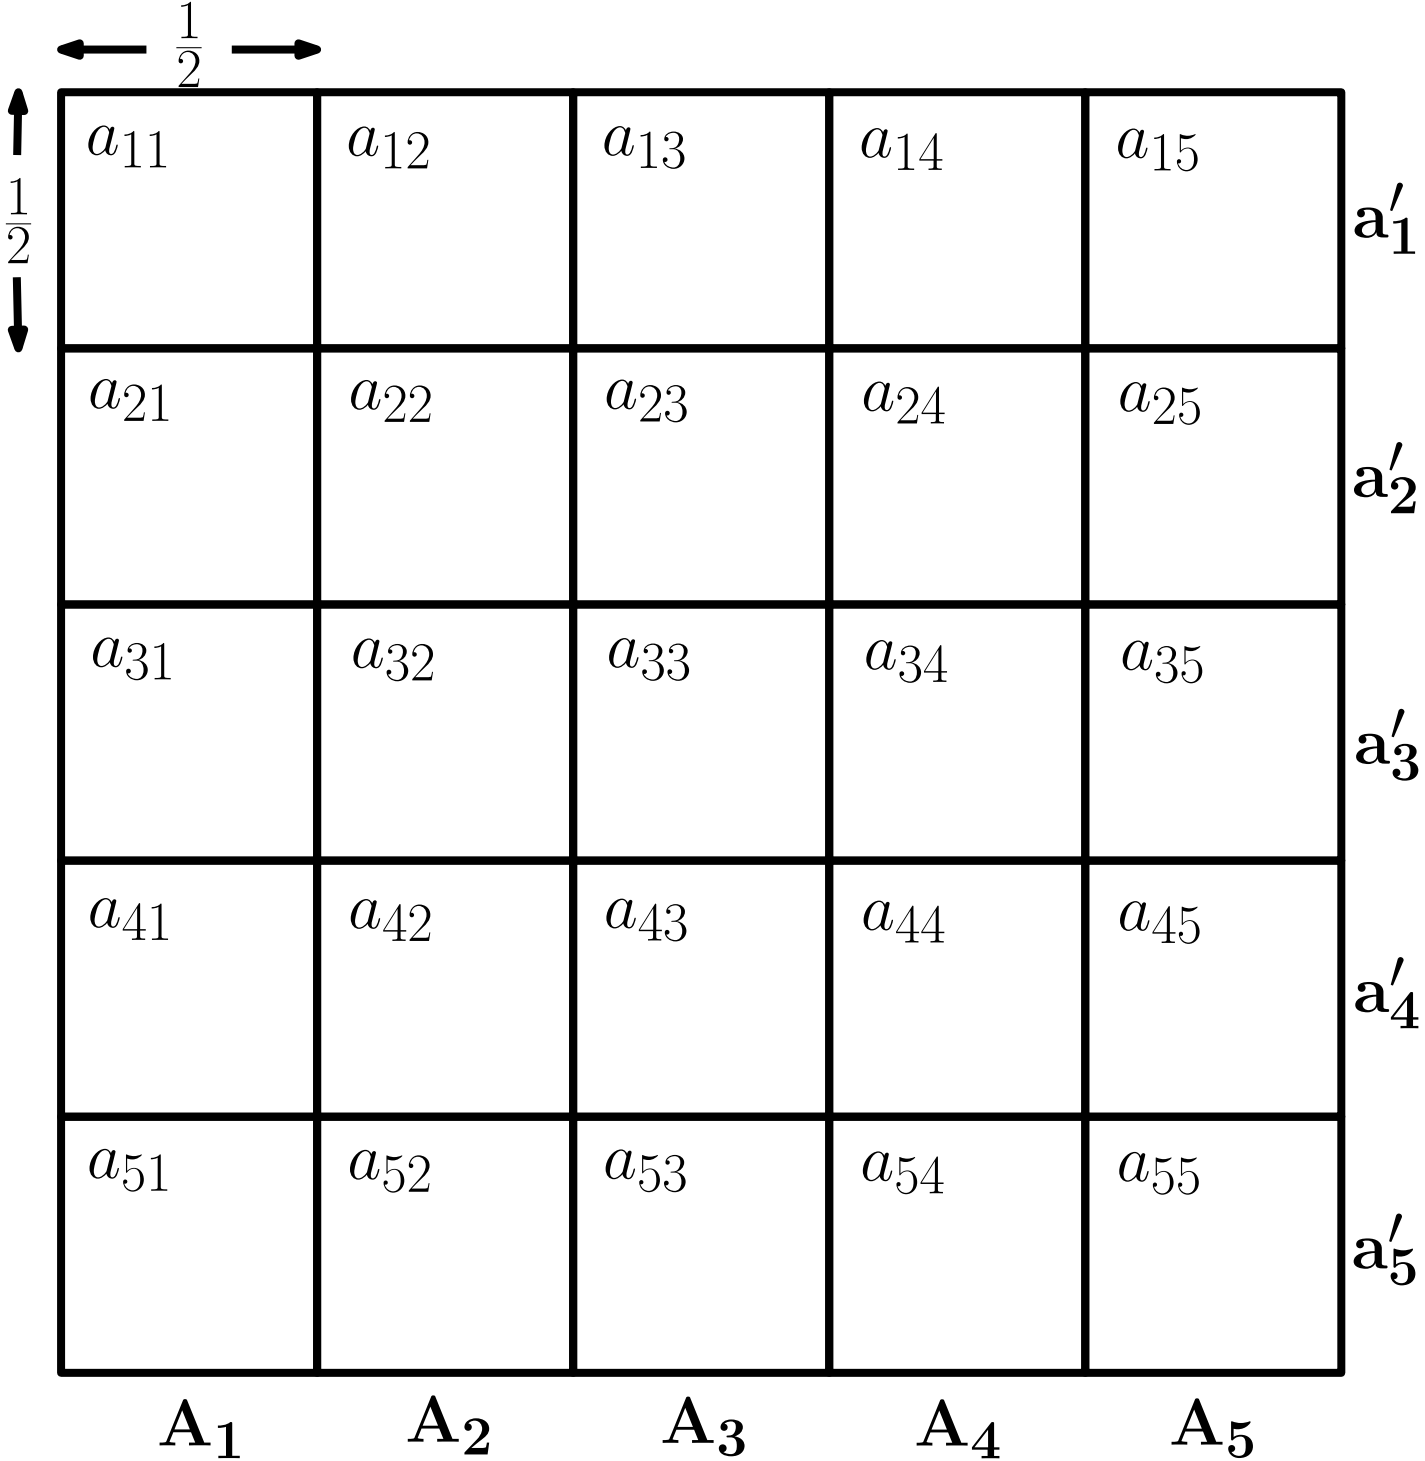

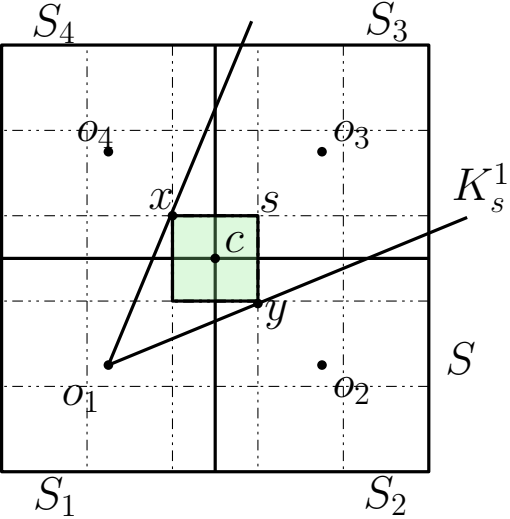

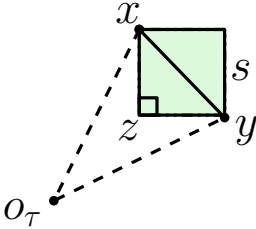

$S'$  $S$  $x$  $s$  $c$  $y$  $o'_1$  $o_1$

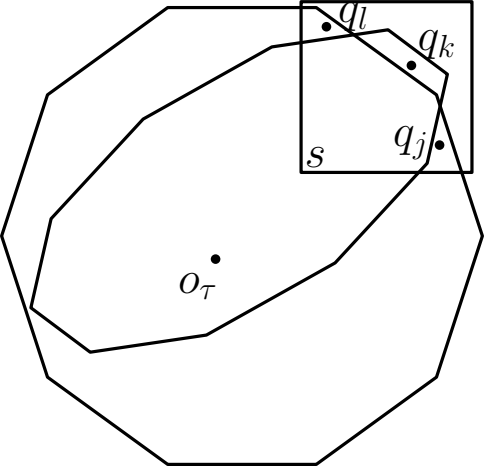

Supplement: Supplementary file 1 [file homothetic_kgons_appendix.pdf]
